# Supplementary material for: Unusual resistance-voltage dependence of nanojunctions during electromigration in ultra-high vacuum
Source: arXiv:1411.0105 source file (2014-11-01)
Supplement: Supplementary file 1 [file stoeffler-final-appendix-rev-6.pdf]

**Supplemental material:**

**Unusual resistance-voltage dependence of nanojunctions during electromigration in ultra-high vacuum**

D. Stöffler,<sup>1</sup> M. Marz,<sup>1, a)</sup> B. Kießig,<sup>2</sup> T. Tomanic,<sup>1</sup> R. Schäfer,<sup>2</sup> H. v. Löhneysen,<sup>1, 2</sup> and R. Hoffmann-Vogel<sup>1</sup>

<sup>1)</sup>*Karlsruhe Institute of Technology, Physikalisches Institut and DFG-Center for Functional Nanostructures, P.O. Box 6980, D-76049 Karlsruhe, Germany*

<sup>2)</sup>*Karlsruhe Institute of Technology, Institut für Festkörperphysik, P.O. Box 3640, D-76021 Karlsruhe, Germany*

---

<sup>a)</sup>Electronic mail: michael.marz@kit.edu

## Appendix A: Details of Sample Preparation

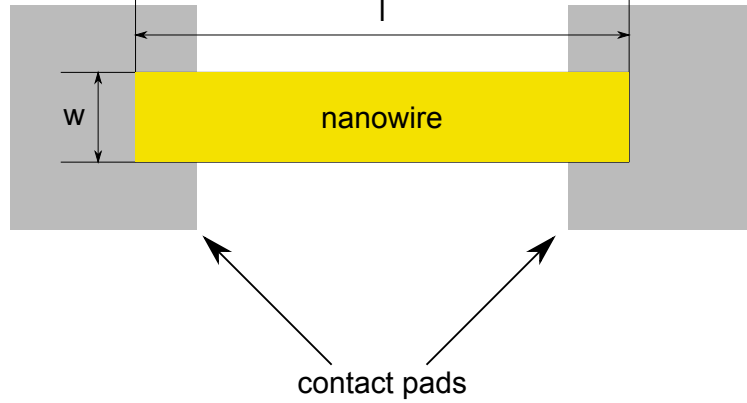

FIG. S1. Sketch of the sample layout for the fabricated nanowires. The typical dimensions were:  $l = 500 - 800$  nm,  $w = 150 - 250$  nm, and  $d = 20 - 30$  nm.

As mentioned in the main text for the sample preparation we used shadow evaporation using either (1) on-chip microstructured  $\text{Si}_{3+x}\text{N}_{4-x}$  membranes or (2) transferable  $\text{Si}_{3+x}\text{N}_{4-x}$  membranes as masks, or (3) electron-beam lithography (EBL) with standard lift-off procedure.

(1) For the preparation of the on-chip  $\text{Si}_{3+x}\text{N}_{4-x}$  membrane masks on a silicon (100) sample with an 800 nm  $\text{SiO}_2$  layer and a 200 nm thick  $\text{Si}_{3+x}\text{N}_{4-x}$  membrane was structured by electron-beam lithography into PMMA to create a substrate with a mask. Then, the substrates were developed and cleaned by reactive ion etching with  $\text{CHF}_3$  and oxygen plasma. This treatment removes the uncovered  $\text{Si}_{3+x}\text{N}_{4-x}$  as well as the remaining PMMA, and all residual organic molecules remaining from the lithography process. Subsequently, the substrate were etched in buffered HF solution to isotropically remove the  $\text{SiO}_2$  layer, and to undercut the remaining parts of the  $\text{Si}_{3+x}\text{N}_{4-x}$  membrane. The process was stopped after etching approximately 400 nm of the  $\text{SiO}_2$  layer resulting in a remaining insulating layer of roughly 400 nm. Afterwards, electric contacts were attached to the substrate surface by gluing gold wires to the  $\text{SiO}_2$  with conductive epoxy adhesive. Finally, the substrates were introduced into the UHV chamber where a metallic layer was evaporated onto the substrates covered with the mask to obtain the desired nanobridge sample. The base pressure was  $1 \cdot 10^{-8}$  Pa for all *in-situ* preparation steps, including shadow evaporation for both manually attached and on-chip masks.

(2) For the transferable  $\text{Si}_{3+x}\text{N}_{4-x}$  membranes, a specially designed UHV-compatible modular holder system that permits performing all preparation steps including contacting *in-situ* was used, for details see Ref. 1.

(3) For the samples prepared by EBL, Si substrates with native oxide ( $\text{SiO}_x \approx 2 - 3 \text{ nm}$ ) were used. In a first EBL step, the nanowire (width  $60 - 150 \text{ nm}$ , length  $300 - 330 \text{ nm}$ , height  $20 - 30 \text{ nm}$ ) was evaporated (in case of Au) or sputtered (in case of Pt) under high vacuum. A second EBL step was performed to fabricate contact leads, details are given in Ref. 2.

As mentioned in the main manuscript the typical dimensions of the nanobridges were:  $w = 150 - 250 \text{ nm}$ ,  $d = 20 - 30 \text{ nm}$ , and  $l = 500 - 800 \text{ nm}$ .

## Appendix B: List of Samples

| sample | material | prep. method | figure                              | $R_{cr}$                 | FN tunneling |
|--------|----------|--------------|-------------------------------------|--------------------------|--------------|
| 1      | Au       | SE           | Fig. 1(a) + Fig. S5                 | $80\ \Omega$             | no           |
| 2      | Al       | EBL          | Fig. 1(b)                           | $480\ \Omega$            | no           |
| 3      | Au       | ME           | Fig. 1(c)+Fig. 1(d)                 | $650\text{-}700\ \Omega$ | no           |
| 4      | Au       | EBL          | Fig. 2 + Fig. S4(b+c)+ Fig. S6(a)   | $600\text{-}800\ \Omega$ | yes          |
| 5      | Au       | EBL          | Fig. S4(a) + Fig. S6(b-d) + Fig. S7 | $> 400\ \Omega$          | yes          |

TABLE I. List of the presented samples that show a crossover from positive to negative slope of  $R(V)$  (SE: shadow evaporation, EBL: electron-beam lithography, ME: mask evaporation). The columns following the sample assignment indicate the material, the preparation method, the figure(s) where the results of the respective sample are shown, the crossover value  $R_{cr}$  from positive to negative slopes of  $R(V)$ , and whether indications of FN tunneling were observed. Sample 4 and 5 denote two different samples prepared on the same chip.

## Appendix C: Proposed contact configuration

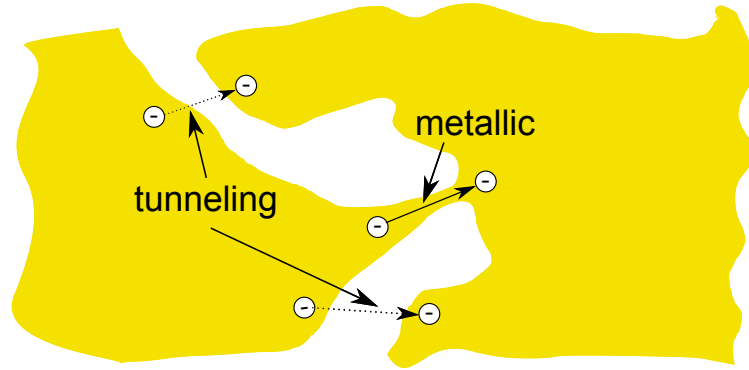

FIG. S2. Sketch of the proposed contact geometry. The contact consists of one metallic connection through which the electrons can pass ballistically (indicated by a solid arrow). Besides this contact the electrons can tunnel at different sites if the distance of the electrodes is small enough (dashed arrow). The overall resistance depends on the metallic constriction and on the tunneling probability, namely the distance and the effective surface of the tunneling electrodes. This model is in agreement with our studies on the morphology changes occurring during EM<sup>3,4</sup>.

## Appendix D: Temperature and voltage dependence of the tunneling contribution

Simmons has shown that the conductance of a tunneling contact in WKB approximation depends on the applied bias voltage<sup>5,6</sup> and on temperature<sup>7</sup> as:

$$G(V, T) = G_V \left(1 + \frac{V^2}{V_0^2}\right) \left(1 + \frac{T^2}{T_0^2}\right) \quad (\text{D1})$$

where  $G$  is the differential conductance and  $G_V$  its value at zero temperature and small  $V$ . According to Simmons  $V_0^2 = 4\hbar^2\varphi/(e^2md^2)$  and  $T_0^2 = 3\hbar^2\varphi/(k_b^2\pi^2md^2)$ , where  $\varphi$  is the effective work function and  $d$  the effective width of the tunneling contact. In the main part of the paper we argue that the conductance of our contacts is partly due to tunneling after some initial phase of the EM process. We take as evidence for tunneling the negative slope of  $R(V)$  which develops after this initial phase. Equation D1 predicts a negative slope as function of  $V$ . Since temperature is risen with increasing  $V$  the  $T^2$  term leads to an additional lowering of  $R$ . Here we show that the contributions included in Eq. D1 are much smaller than the nonlinearities in the  $I/V$ -characteristics we observe in our experiments and are thus not the main cause for the negative slope in  $R(V)$ . At the end of this section we develop a simple model which includes variations of the distance  $d$  over which electrons tunnel. If a small slit of width  $d$  is formed in the EM process, thermal expansion of the electrodes on both sides of this slit or the electrostatic field increasing with voltage leads to significant variations of  $d$  as a result of self heating in response to increasing bias. We show that with reasonable model parameters this variation will lead to the observed nonlinearities in the  $I/V$ -characteristics.

To gain further insight we first use Simmons theory to estimate model parameter for the observed conductance at low bias,  $G_V$ . The WKB expression is according to Simmons<sup>5,6</sup>:

$$G_V = A\sqrt{2m\varphi}e^2/(4\pi^2\hbar^2 \cdot d) \exp(-d\sqrt{8m\varphi}/\hbar), \quad (\text{D2})$$

where  $A$  is the effective cross section of the tunneling contact. Equation D2 can be inverted to yield

$$d = \hbar W\left(\frac{e^2m\varphi A}{G_V\pi^2\hbar^3}\right) / \sqrt{8m\varphi}, \quad (\text{D3})$$

with  $W(x)$  labeling the zero branch of the Lambert function. Thus, the unknown distance  $d$  we want to estimate depends on the work function (which we set to the literature value

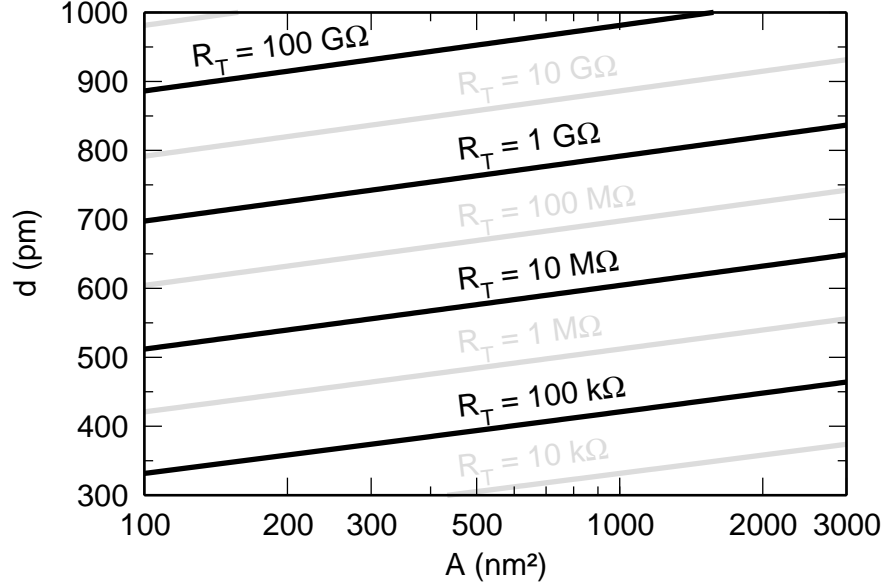

FIG. S3. Effective tunneling distance  $d$  (see Eq. D3) as a function of the effective area  $A$  of the tunneling contact for various tunneling resistances  $R_T$ . The distance  $d$  is displayed in the range from  $d = 300$  pm (close to the literature value  $d = 288$  pm for the nearest neighbor distance in gold) to  $d = 1$  nm. The area  $A$  varies between  $A = 10$  nm  $\times$  10 nm and  $A = 30$  nm  $\times$  100 nm, i. e. the almost full cross section of the initial nanobridge used in our experiments. Reasonable values for  $d$  are found at  $R_T > 100$  k $\Omega$ .

for gold here,  $\varphi_{lit} = 5.1$  eV [8 and 9]), the effective tunneling cross section  $A$ , and the tunneling conductance  $G_V = 1/R_T$ . Equation D3 is visualized in Fig. S3, where we plot  $d$  as a function of the effective cross section  $A$  for various values of  $R_T$ . If we assume that the total conductance of the partially electromigrated structure is comprised of a metallic part in parallel to the tunneling contribution, we can write  $R_{total}/R_T = p$ , where  $p$  measures the percentage of the tunneling contribution. In our experiment we find the crossover to a negative slope in  $R(V)$  well below  $R_{total} = 1$  k $\Omega$ . In view of the numbers derived for Fig. S3, it is evident that the tunneling contribution is at most a few percent in our experiments presumably increasing when the resistance goes up in the course of EM induced thinning. The effective distance  $d$  does not depend strongly on the tunneling resistance or the tunneling area. A value of the order of  $d = 500$  pm seems to be a reasonable estimate.

With this value at hand, we can calculate the nonlinearity parameters  $V_0$  and  $T_0$  in Eq. D1. We get  $V_0 = 2.5$  V and  $T_0 = 8000$  K. The correction due to temperature increase is

small even under extreme conditions (1.5 % at 1000 K) and can be ignored. For the voltage dependence of  $R(V)$  we get

$$R^{-1}(V) = G_V \left( 1 + p \cdot \frac{V^2}{V_0^2} \right). \quad (\text{D4})$$

This equation predicts for  $V = 1$  V a change of the order of  $0.16 \cdot p$  only. The experimentally observed changes (see, e. g., Fig. S4) are at least two orders of magnitude larger.

We now discuss the influence of thermal expansion on the tunneling conductance and develop, to this end, a simple model on the basis of Eq. D2. Changes in  $d$  will change  $G_V$  primarily due to the exponential factor in Eq. D2,

$$G_V(d - \Delta d) \approx G_V(d) \exp(\Delta d \sqrt{8m\varphi}/\hbar), \quad (\text{D5})$$

where the notation  $G_V(d)$  emphasizes the dependence of  $G_V$  on the distance  $d$ .

The temperature close to the tunneling contact is a function of the applied bias and could reach several hundred Kelvin before structural changes are induced by EM. While thermal expansion of the metallic film leads only to an increasing thickness in regions several tens of nm away from its boundaries, grains adjacent to a boundary can expand freely to the side as well. Estimating the typical grain diameter  $D$  to be of the order of the initial film thickness  $D \approx 30$  nm and using the thermal expansion coefficient of gold at room temperature  $\alpha_{\text{Au}} = 14.2 \cdot 10^{-6} \text{ K}^{-1}$  [10], we get for a typical temperature enhancement by  $\Delta T = 300$  K,

$$\Delta d \approx D \alpha_{\text{Au}} \Delta T = 128 \text{ pm}$$

This leads according to Eq. D5 to an increase of the tunneling contribution to the conductance by a factor of almost  $\exp(128 \text{ pm} \sqrt{8m\varphi}/\hbar) \approx 20$ . Therefore, even if the tunneling contribution  $p$  is small, considerable changes in the total conductance  $R(V)$  are expected. A similar large distance change could occur by relaxations due to the electrostatic field.

For a more explicit estimate we approximate the temperature enhancement by<sup>11</sup>  $\Delta T \approx \gamma V$  with a phenomenological proportionality constant  $\gamma$ . Attributing changes in  $d$  solely to thermal expansion leads then to

$$G_V(V) = G(0) \exp(\beta^* V),$$

where  $\beta^* = D\alpha_{\text{Au}}\gamma\sqrt{8m\varphi}/\hbar$  is again a phenomenological fitting variable. For the voltage dependence of the measured resistance we get finally:

$$R(V) = \frac{R(V=0)}{1 + p(\exp(\beta^*V) - 1)} \quad (\text{D6})$$

Equation D6 is used in Fig. S4 to fit experimental data of several EM cycles. Despite its simplicity, the model gives a reasonable description of the data with adequate model parameters. A similar analysis could be done in terms of the model by Brinkman *et al.*<sup>12</sup>, which was also used in Ref. 13.

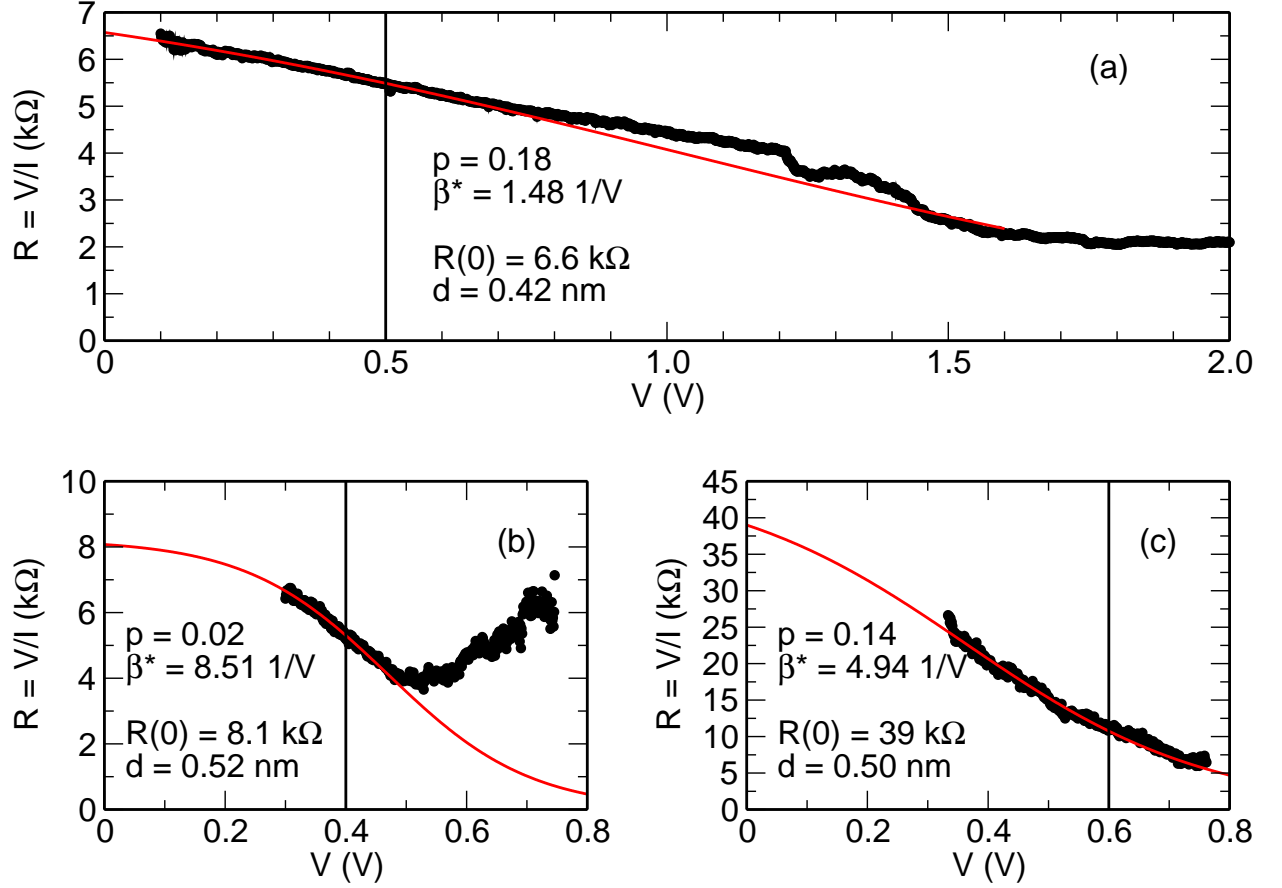

FIG. S4. Resistance vs. voltage data of different EM cycles (black) on two Au bridges (sample 4 and 5) fabricated by electron beam lithography on the same chip. The full EM process of sample 4 is shown in Fig. 2(a). To explain the large decrease of the resistance, thermal and/or electrostatic expansion has been included in our model for the fits (red). The vertical line in all panels shows the cutoff used for the fits. We are able to fit the data and determine besides the barrier width  $d$ , the proportion  $p$  of the tunneling to the full conductance. For calculating the tunneling barrier a value of  $\varphi_{lit} = 5.1$  eV for the work function of Au<sup>8,9</sup> has been used and an effective tunneling area of  $A_{cros} = 3000$  nm<sup>2</sup> has been assumed. The obtained tunneling barrier and tunneling contributions are (a)  $d = 0.42$  nm,  $p = 0.18$ , (b)  $d = 0.52$  nm,  $p = 0.02$  and (c)  $d = 0.50$  nm,  $p = 0.14$

## Appendix E: Resistance vs. differential resistance

We emphasize that the negative slopes observed in  $R(V) := V/I$  should not be confused with negative differential resistance  $R_{\text{diff}} := dV/dI$ . To clarify this point, we have plotted in Fig. S5 the applied voltage  $V$  as function of the measured current  $I$  for the sample shown in Fig. 1(a).

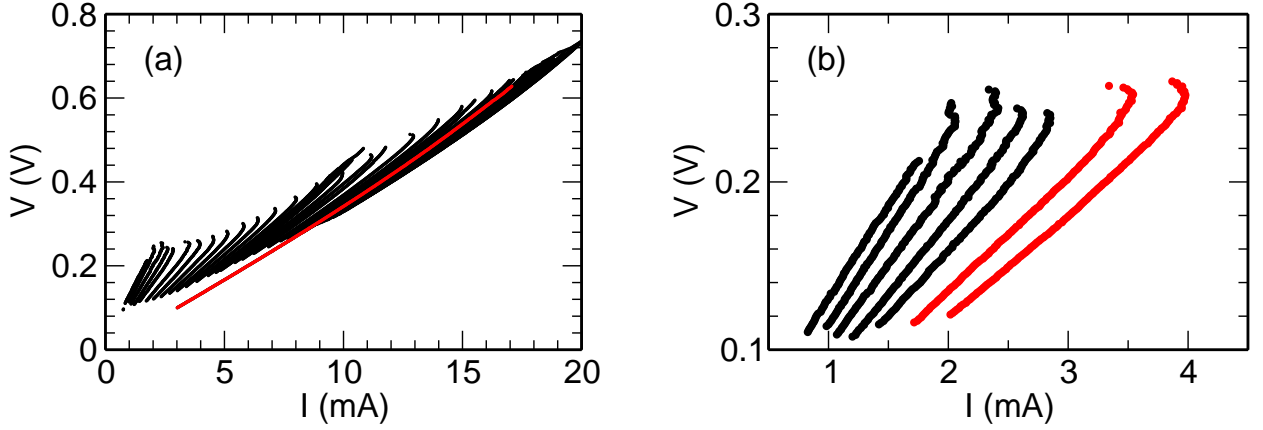

FIG. S5. Applied voltage as function of the measured current. (a) All electromigration cycles for the sample shown in Fig. 1(a). The first cycle after a second deposition step is plotted in red. (b) Detail of the crossover between positive slope in  $R(V)$  vs.  $V$  (red) to negative slopes (black).

Fig. S5(a) shows the results of the full EM protocol, where only small changes are seen from one cycle to the next. The very first cycle (red) after the second deposition step<sup>17</sup> is noticeably different from the following ones since, during the first cycle, an annealing of grain boundaries and/or defects is likely to occur. The cycles where the crossover between positive and negative slope in  $R(V)$  occur are displayed on an enlarged scale in Fig. S5(b). Clearly, the differential resistance ( $dV/dI$ ) stays positive, except at the very end of the cycles where the thinning of the contacts happens. However, for the last five cycles, plotted in black, the slope increases substantially compared to the two cycles before, shown in red.

## Appendix F: Fowler-Nordheim (FN) plots

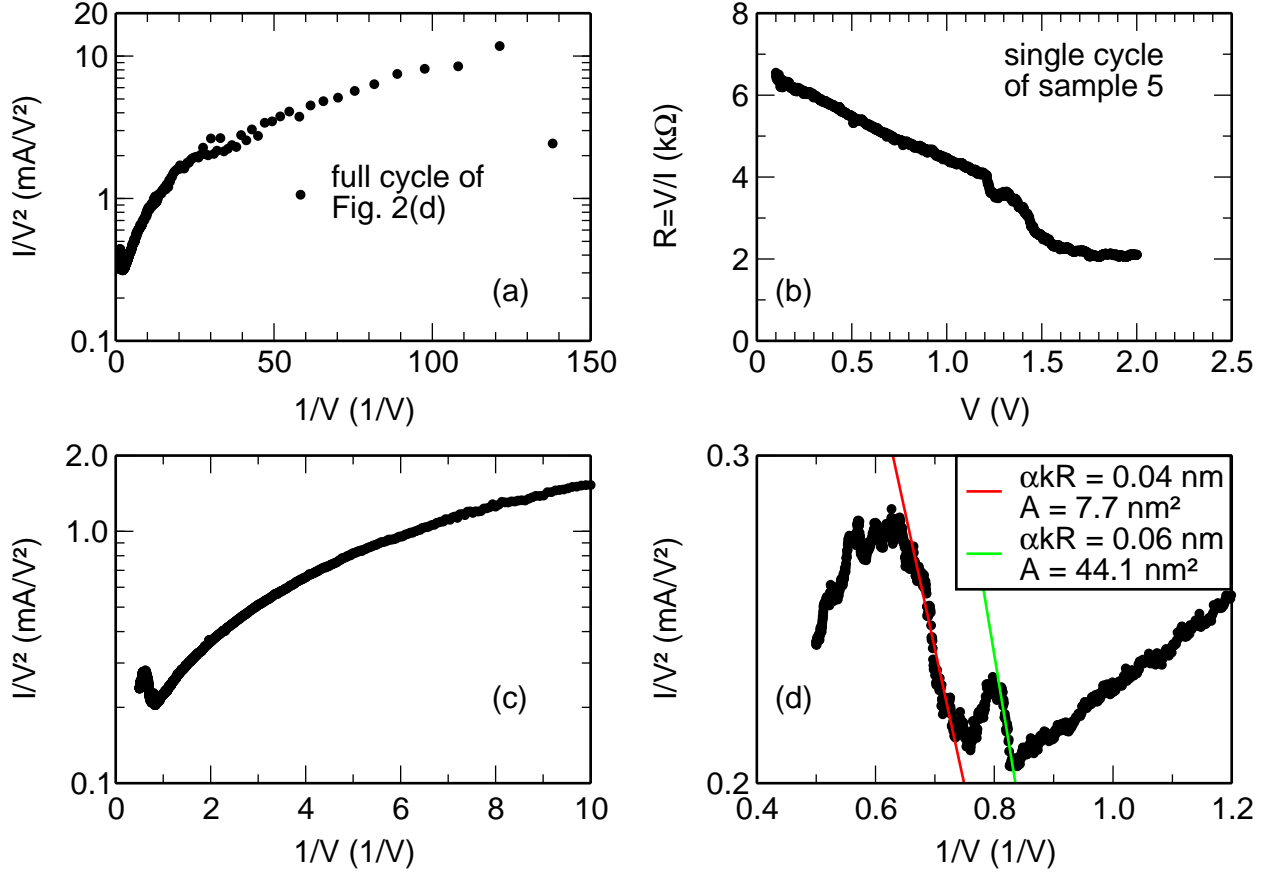

FIG. S6. (a) Full-scale FN plot of Fig. 2(d) (sample 4, see Fig. S4). (b)  $R(V)$  cycle of sample 5 with  $R(0.2 \text{ V}) \approx 6 \text{ k}\Omega$ . (c) Corresponding FN plot of (b). Both FN plots suggest a transition from direct tunneling to Fowler-Nordheim tunneling below  $\approx 1 \text{ V}^{-1}$ . (d) Detail for high bias of (c) including two possible linear fits and the resulting values for  $\alpha kR$  and  $A$ . For  $V \gtrsim 1.8 \text{ V}$  a sharp drop occurs, which we attribute to sudden changes in the contact region due to field emission. In this case, we speculate that the contact has changed either by the diffusion of a larger cluster within the contact or by blunting of the contact. In both cases we would expect a lower starting resistance for the following cycle, which is what we observe, see Fig. S7(a).

Following the calculations of Müller *et al.*<sup>14</sup> the current-voltage dependance in the WKB approximation can be rewritten as:

$$I \propto V \exp \left( -\frac{2d\sqrt{2m_e\varphi}}{\hbar} \right)$$

or, equivalently, as:

$$\ln \frac{I}{V^2} \propto \ln \left( \frac{1}{V} \right) - \frac{2d\sqrt{2m_e\varphi}}{\hbar},$$

leading to a logarithmic growth as signature of direct tunneling in a  $\ln I/V^2$  vs.  $1/V$  plot.

In contrast, the FN tunneling characteristics reads as:

$$\ln \frac{I}{V^2} \propto \frac{4d\sqrt{2m_e\varphi^3}}{3\hbar e} \left( \frac{1}{V} \right)$$

showing a linear behavior with positive slope in the  $\ln I/V^2$  vs.  $1/V$  plot. The plots in Fig. S6(a) and (c) show that some of our data display characteristics that are typical for the transition from direct tunneling to FN tunneling<sup>14–16</sup>. As soon as the contact resistance is changed our EM thinning algorithm starts a new cycle at low bias. Therefore, we are not able to measure a reversible branch of the current-voltage characteristic which would be desirable for an assignment to FN tunneling. Fig. S7 shows the evolution of  $R(V)$  and  $I(V)$  around the cycle displayed in Fig. S6(d) here tagged ' $n$ '. For  $n + 1$  a smaller resistance is found due to an uncontrolled change caused by field emission.

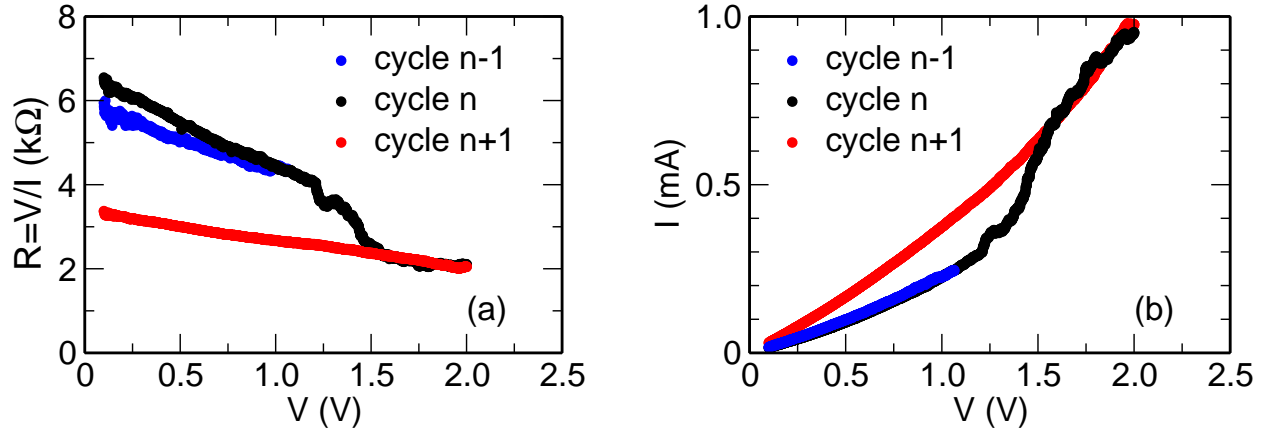

FIG. S7. (a)  $R(V)$  of the cycle ( $n$ ), plotted in Fig. S6(b), as well as, the previous cycle ( $n - 1$ ) and the following cycle ( $n + 1$ ). For cycle  $n - 1$  the voltage was not large enough to reach the field-emission regime. For cycle  $n$  field emission was reached and the contact changed due to the diffusion of a larger cluster or blunting. The initial resistance  $R(V_{min})$  for cycle  $n + 1$  is significantly lower than for cycle  $n$  and  $n - 1$ . At high bias the end resistance of cycle  $n$  is again reached, indicating that a stable contact was formed. (b) Corresponding  $I(V)$  plots. For cycle  $n + 1$  no transition to the FN tunneling is observed, i.e., no significant increase in the slope is found.

## REFERENCES

- <sup>1</sup>C. Gärtner, R. Hoffmann, F. Pérez-Willard, M. Sauter, C. Sürgers, H. v. Löhneysen, Rev. Sci. Instr. **77**, 026101 (2006).
- <sup>2</sup>R. Hoffmann, D. Weissenberger, J. Hawecker and D. Stöffler, Appl. Phys. Lett. **93**, 043118 (2008).
- <sup>3</sup>D. Stöffler, S. Fostner, P. Grütter, and R. Hoffmann-Vogel, Phys. Rev. B **85**, 033404 (2012).
- <sup>4</sup>D. Stöffler, Ph.D. thesis, Karlsruhe Institute of Technology, Karlsruhe 2012.
- <sup>5</sup>J. G. Simmons J. Appl. Phys. **34**, 238 (1963).
- <sup>6</sup>J. G. Simmons J. Appl. Phys. **34**, 1793 (1963).
- <sup>7</sup>J. G. Simmons J. Appl. Phys. **35**, 2655 (1964).
- <sup>8</sup>A. Eberhagen, Fortschr. d. Phys. **8**, 245 (1960).
- <sup>9</sup>H. Landolt and R. Börnstein, *Landolt-Börnstein: Numerical Data and Functional Relationships in Science and Technology*, New Series, edited by W. Martienssen, (Springer, New York, 2011).
- <sup>10</sup>D. R. Lide, *CRC-Handbook of Chemistry and Physics*, 76th Edition (CRC, Boca Raton, 1995).
- <sup>11</sup>R. Holm, Electric Contacts, Springer-Verlag, Berlin (1967).
- <sup>12</sup>W. F. Brinkman, R. C. Dynes, and J. M. Rowell, J. Appl. Phys. **41**, 1915 (1970).
- <sup>13</sup>A. v. Bieren, A. K. Patra, S. Krzyk, J. Rhensius, R. M. Reeve, L. J. Heyderman, R. Hoffmann-Vogel, and M. Kläui, Phys. Rev. Lett. **110**, 067203 (2013).
- <sup>14</sup>M. Müller, G.-X. Miao, and J. S. Moodera, Europhys. Lett. **88**, 47006 (2009).
- <sup>15</sup>R. H. Fowler, and L. Nordheim, Proc. R. Soc. London, Ser. A **119**, 173 (1928).
- <sup>16</sup>M. L. Trouwborst, C. A. Martin, R. H. M. Smit, C. M. Guedon, T. A. Baart, S. J. van der Molen, and J. M. van Ruitenbeek, Nano Lett. **11**, 614 (2011).
- <sup>17</sup>After the first metal deposition the sample was completely burned through by controlled EM cycles. In a second metal deposition step the formed gap was closed again.
